# Supplementary material for: Genetic Meta-Structure Search for Recommendation on Heterogeneous Information Network
Source: arXiv:2102.10550 source file (2021-02-21)
Supplement: Supplementary file 1 [file Appendix.tex]

\appendix
\section{Appendix for Reproducibility}\label{sec:Appendix}
To answer the committee's call to promote the reproducibility of research, we provide additional details on experiments and model interpretation in this section. 

\subsection{Training and Learning}
In GEMS, the multi-view GCN is trained in a supervised learning way with the purchase record of dataset $\mathcal{D} = \{<v_u,v_i>\}$, where $v_u$ stands for users ans $v_i$ stands for items. The specific meaning of the item depends on the dataset. The recommendation likelihood is calculated as follows:
\begin{equation}
    z(v_u,v_i) = \sigma \big(y_{v_u} \cdot y_{v_i} \big),
\end{equation}
where $y_{v_u}, y_{v_i}$ are fused embeddings of the GCN backend, and $\sigma(\cdot)$ is the sigmoid activation function. 

For any positive purchase record in dataset $\mathcal{D}$, we sample a pre-defined number of negative items $v_n$ according to the occurrence frequency of items. We adopt a max-margin based ranking loss function to train the GCN backend as follows:
\begin{equation}
J_{\mathcal{G}}(v_u, v_i) = \mathbb{E}_{v_n}\mathrm{max}\left\{0,\ z(v_u, v_n)-z(v_u, v_i)+\Delta \right\},
\end{equation}
where $\Delta$ denotes the hyper-parameter of pre-defined margin. The intuition of this loss function is to train the model to predict the positive samples with a higher likelihood by a pre-defined margin than negative items.

An important feature of GEMS is that, individuals are fully independent after crossover operation. In that case, meta-graph adjacency search and GCN training can be fully paralleled. This feature enables us to leveraging the high concurrency ability of modern computing hardware to speed-up model convergence.

\subsection{Parameter Sensitivity}
We investigate the sensitivity of parameters for GEMS model on regularization parameters and embedding dimension. Experiments are implemented on Yelp dataset.

From Figure \ref{fig:param}, we can observe that the performance varies with regularization parameters (lambda) and the embedding dimensions, but the NDCG@10 consistently remains above 0.16. Specifically, the optimal regularization parameter for GEMS is 0.05. In addition, the NDCG@10 consistently increases from $0.1714$ to $0.1959$ when the embedding dimensions increase from $16$ to $64$, and it starts to go down when the embedding dimensions are 128. This phenomenon validates the hyper-parameter choices during experiment section. 
 
Another important hyper-parameter is learning rate. For GEMS model and all other baselines, we adopt a variable strategy that uses relatively high learning rate during warm-up phase, then decreases the learning rate in an exponential decay. Combined with ADAM optimizer, our implementation is not sensitive on learning rate choices given enough initial learning rate and warm-up period.

\subsection{Deployment Details}
We implement our model and comparison baselines with pytorch. All the evaluated models are implemented with Pytorch, and trained on a server with 32 core CPU (AMD Ryzen Threadripper 2990WX) and four GPUs (NVIDIA GeForce RTX 2080Ti * 4). Empirically, we observe the GEMS can be effectively trained in less than 2 days. Since each individuals are completely independent during model training, we can fully leverage the high concurrency of modern hardware to speed-up computing efficiency.

\begin{figure}[H]
 \centering
  %\vspace{-0.15in}
    \subfigure[Regularization]{
         \label{fig:lamb}
         \includegraphics[width=.23\textwidth]{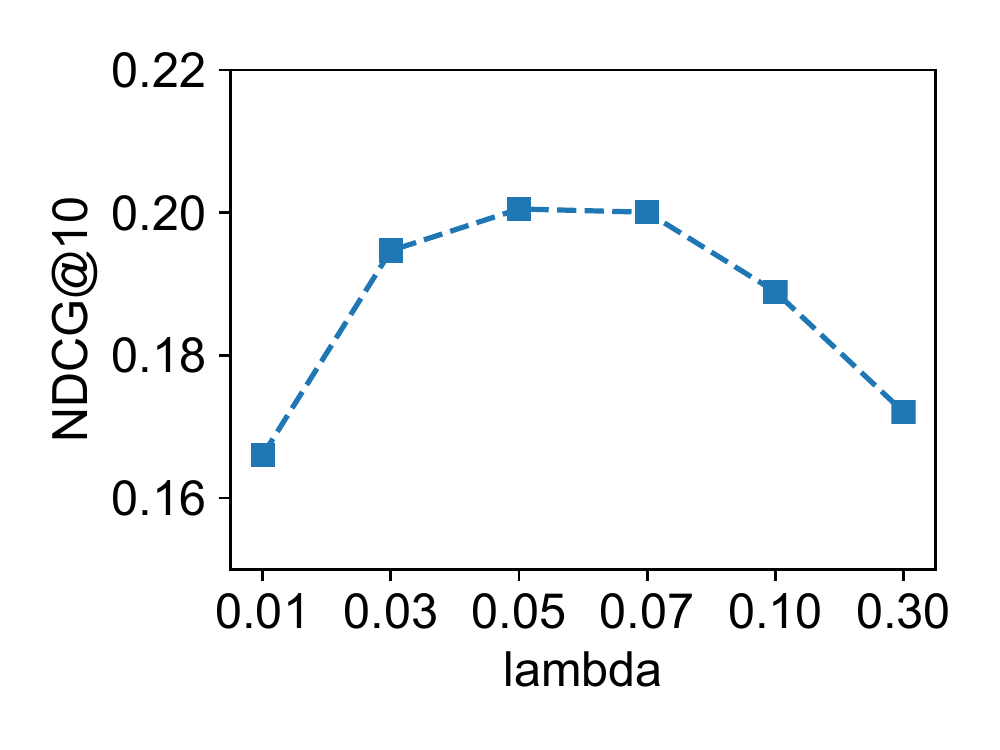}}
    \subfigure[Embedding size]{
        \label{fig:emb}
        \includegraphics[width=.23\textwidth]{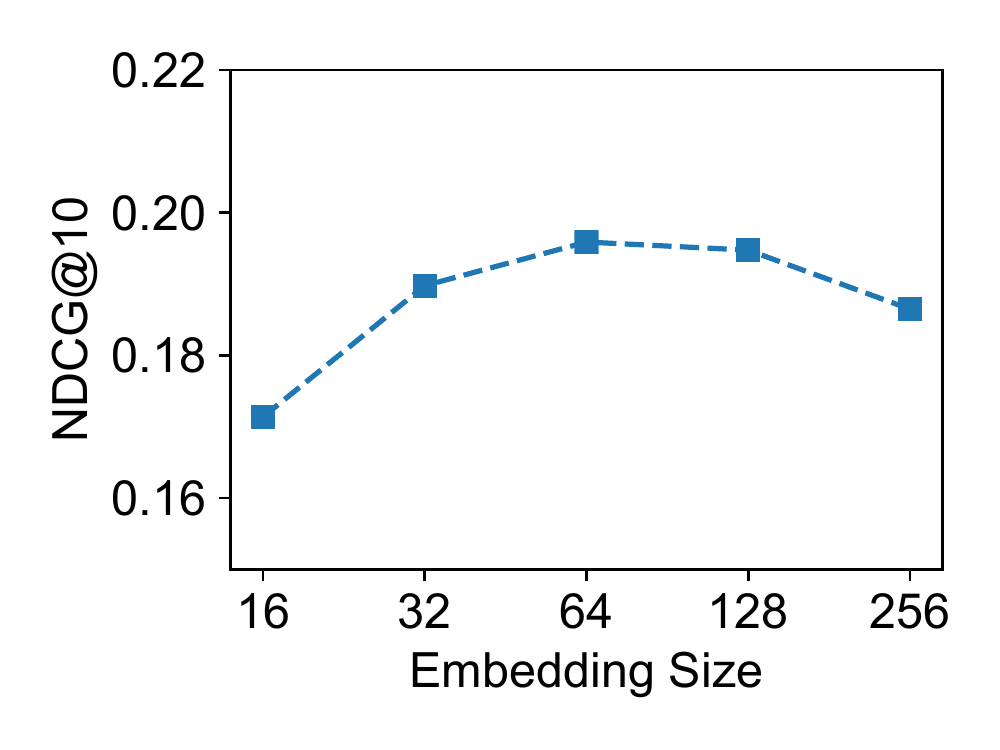}}
 \caption{Parameter sensitivity on Yelp dataset.}
% \vspace{-0.2in}
 \label{fig:param}
\end{figure}

% \textbf{Extra experiments for evaluating meta-graph predictor.} Here, we demonstrate the predictor performance on the other two selected datasets.
% \begin{figure}[!h]
%  \centering
%   %\vspace{-0.15in}
%     \subfigure[Training result on Yelp dataset]{
%         \label{fig:pred_tr_yelp}
%         \includegraphics[width=0.23\textwidth]{figures/pred_yelp_train.pdf}}%
%     \subfigure[Training result on Douban movie dataset]{
%         \label{fig:pred_tr_douban}
%         \includegraphics[width=0.23\textwidth]{figures/pred_douban_train.pdf}}\\
%     \vspace{-0.1in}
%     \subfigure[Testing result on Yelp dataset]{
%         \label{fig:pred_test_yelp}
%         \includegraphics[width=0.23\textwidth]{figures/pred_yelp_test.pdf}}
%     \subfigure[Testing result on Douban movie datset]{
%         \label{fig:pred_test_douban}
%         \includegraphics[width=0.23\textwidth]{figures/pred_douban_test.pdf}}%
%         \vspace{-0.1in}
%  \caption{Effectiveness of meta-graph predictor on other datasets}
% % \vspace{-0.2in}
%  \label{fig:predictor_more}
% \end{figure}

\subsection{Algorithm Procedure} To better understand the procedure of GEMS, we provide a pseudo-code as follows. 

\begin{algorithm}
\caption{: Genetic Meta-graph Search}\label{alg:gems}
\begin{algorithmic}[1]
\REQUIRE{HIN $G=(\mathcal{V}, \mathcal{E})$, Dataset $\mathcal{D}=\left\{<v_u, v_i>\right\}$, node features $\left\{\mathbf{x}_v, \forall v\in V \right\}$, epoch number $e$}
\ENSURE 
\STATE Initialize  $genePool$ for the $population$
\STATE Initialize meta-graph predictor $predic(\cdot)$
\FOR{$epoch=1$ to $e$} 
\STATE /*Mutate and Crossover*/
\STATE $genePool$ = Mutate$(genePool)$ 
\STATE $genePool$ = Crossover$(genePool)$ 
\FOR{$individual$}
\STATE Assign $individualGenes$ from $genePool$
\STATE /*Using predictor to filter promising individuals*/
\IF{$predic(individualGenes)<threshold$} 
\STATE $metric$ = $predic(individualGenes)$
\STATE continue
\ELSE
\FOR{$gene$ in $individualGenes$}  
\STATE /*Adjacency Search*/
\STATE $\mathcal{N}_{gene} = \mathrm{AdjSearch}(gene) $
\ENDFOR 
\STATE /*Train the GCN and preform recommendation task*/
\STATE $metric$ = GCN($\mathbf{x}_v,\mathcal{D},\mathcal{N}$)
\ENDIF
\ENDFOR 
\STATE /*Eliminate and Reproduce*/
\STATE $population$ = Eliminate($population,metrics$)
\STATE $population$ = Reproduce($population,metrics$)
\STATE Train meta-graph predictor by $(individual, metric)$ pairs

\ENDFOR 
\end{algorithmic}
\end{algorithm}
